# Supplementary material for: Exponentially Tilted Thermodynamic Maps (expTM): Predicting Phase Transitions Across Temperature, Pressure, and Chemical Potential
Source: arXiv:2503.15080 ancillary file (2025-03-19)
Supplement: Supplementary file 1 [file supplement.pdf]

# Exponentially Titled Thermodynamic Maps (expTM): Predicting Phase Transitions Across Temperature, Pressure, and Chemical Potential


Suemin Lee# and Lukas Herron

*Biophysics Program and Institute for Physical Science and Technology,*
*University of Maryland, College Park 20742, USA and*
*University of Maryland Institute for Health Computing, Bethesda, Maryland 20852, USA*

Ruiyu Wang#

*Institute for Physical Science and Technology,*
*University of Maryland, College Park 20742, USA*

Pratyush Tiwary*

*Biophysics Program and Institute for Physical Science and Technology,*
*University of Maryland, College Park 20742, USA*
*University of Maryland Institute for Health Computing,*
*Bethesda, Maryland 20852, USA and*
*Department of Chemistry and Biochemistry and*
*Institute for Physical Science and Technology,*
*University of Maryland, College Park 20742, USA*



(Dated: March 19, 2025)

## I. EXPONENTIALLY TILTED THERMODYNAMICS MAPS ALGORITHM

Here, we present a short algorithm of Exponentially tilted Thermodynamics Maps (expTM), which integrates thermodynamic control variables such as temperature ($\beta$) and another thermodynamic parameter of interest such as pressure or chemical potential ($\alpha$) into a unified framework. The workflow begins by preparing input features with the associated thermodynamic conditions. Once it is prepared, the expTM model is then trained to map the data to an exponentially tilted Gaussian prior, where the tilting adjusts the prior distribution's mean and variance according to $\alpha$ and $\beta$, respectively. Finally, new samples are generated by reversing the diffusion process, allowing the model to generate new configurations under arbitrary thermodynamic conditions.

---

**Algorithm 1** Exponentially Tilted Thermodynamic Maps (expTM) with $(\alpha, \beta)$ Terms

---

**Step 1: Data preparation.**

- Input feature configurations (or structures) $\{\mathbf{x}_i\}_{i=1}^N$
- Thermodynamic parameters $\{T_i, \alpha_i\}_{i=1}^N$ (e.g., temperature $T_i$ and pressure/chemical potential $\alpha_i$)

Assign each configuration $\mathbf{x}_i$ its corresponding temperature $T_i$. Combine all configurations into a set $\big\{(\mathbf{x}_i, T_i, \alpha_i)\big\}_{i=1}^N$.

**Step 2: Estimate or initialize $\beta_i^{(j)}$ and $\alpha_i^{(j)}$.**

**(a)** **If** linear fluctuations are assumed:
$\beta_i^{(j)} \leftarrow \mathrm{Var}\big[\mathbf{x}_m^{(i)}\big]^{-1}, \quad \alpha_i^{(j)} \leftarrow \mathbb{E}\big[\mathbf{x}_m^{(i)}\big].$

**(b)** **Else** keep them fixed at the input values:
$\beta_i^{(j)} = \beta, \quad \alpha_i^{(j)} = \alpha.$

**Step 3: Train the expTM model.**

**(a)** Define a new *exponentially tilted Gaussian prior*,
$\mathbf{z} \sim \exp\Big(-\frac{\beta}{2}\big(\mathbf{z}-\alpha\big)^2\Big).$

**(b)** Use score-matching to learn $(\mathbf{x}, \beta, \alpha) \mapsto \nabla_{\mathbf{x}} \log p(\mathbf{x} \mid \beta, \alpha)$, so the forward and reverse SDEs connect data $\mathbf{x}_m^{(i)}$ and prior distribution $p(\mathbf{z})$.

**(c)** Minimize the training loss to ensure that samples drawn from the tilted prior are correctly mapped to target data distributions at $p(\mathbf{x}|\beta_i, \alpha_i)$.

**Step 4 : Generate New Samples.**

- Sample $\widetilde{\mathbf{z}}$ from the tilted prior at new $(\beta^*, \alpha^*)$.
- Apply reverse diffusion to sample $\widetilde{\mathbf{x}} \sim p(\mathbf{x}|\beta^*, \alpha^*)$.

**Output:** A trained expTM model can generate samples at any $(T^*, \alpha^*)$.

---

* ptiwary@umd.edu

## II. GRAND CANONICAL LATTICE GAS MODEL

The grand canonical lattice gas model described in the main text was studied using Monte Carlo (MC) simulations on a $20 \times 20$ square lattice. A total of 20,000 training samples were generated, comprising 10,000 configurations each at low and high temperatures. MC simulations ensure that configurations at a given temperature and chemical potential are sampled from the equilibrium distribution, accurately reflecting the conditions of the bath. The sampled output ranges from 0 to 1, representing the occupation probability of an atom at each lattice site.

Figure S1(a) illustrates the variations in lattice configurations under different pressures and chemical potentials, while Fig.S1(b) shows the evolution of the system's density averaged over 5,000 samples across various temperatures and chemical potentials.

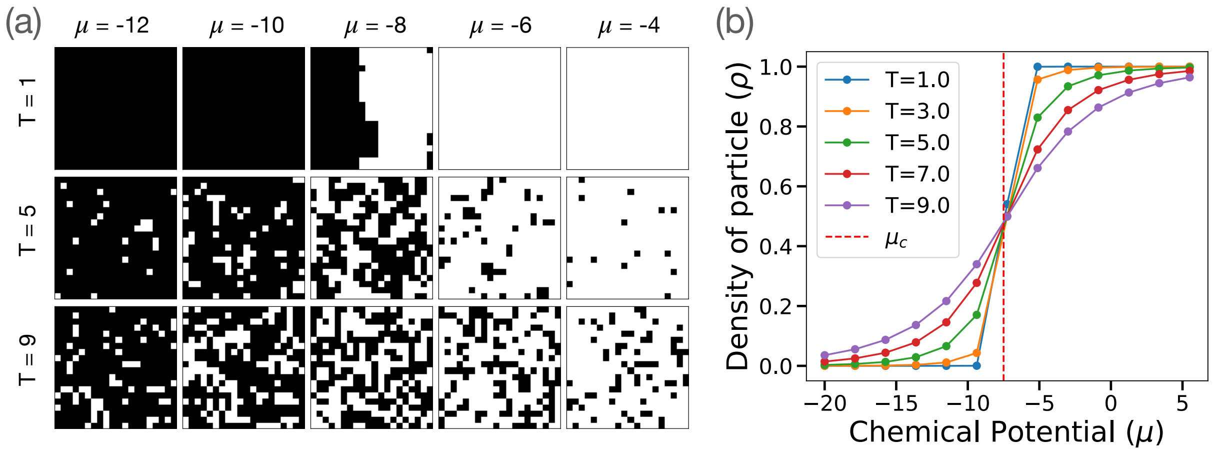


FIG. S1. Grand canonical Monte Carlo simulations of a $20 \times 20$ lattice gas at various pressures, chemical potentials, and temperatures: (a) representative configurations and (b) density change over averaged 10,000 samples.

## III. ADDITIONAL SETTINGS AND RESULTS OF PHASE TRANSITION OF $CO_2$

### A. Molecular dynamics simulations settings

The settings of molecular dynamics (MD) simulations for $CO_2$ are based on prior work.[S1] All simulations are performed using GROMACS 2022.3,[S2, S3] with each simulation containing 256 $CO_2$ molecules. The force field parameters for $CO_2$ are described in Table S1. To address simulation instabilities arising from the linear geometry of $CO_2$, two dummy atoms are added at a distance of $d_{CM} = 0.098925\,\text{nm}$ and with a mass of 22 using the *virtual_sites2* keyword in GROMACS. The distance between the dummy atoms, $M1$ and $M2$, is constrained to 0.19785 nm using the *constraint* keyword in GROMACS. Simulations are conducted in the isothermal–isobaric (NPT) ensemble. The temperature is maintained at 350 K using the velocity-rescaling thermostat method with a relaxation time of 0.1 ps.[S4] The pressures are set to 1, 3, 5, and 8 GPa across four simulations controlled by the Berendsen coupling algorithm.[S5] The compressibility is set to $10^{-5}\,\text{bar}^{-1}$. Each simulation runs

for 500 ns with a time step of 2 fs. All bonds within the $CO_2$ molecules are constrained using the LINCS algorithm.[S6]

TABLE S1. Force field parameters for $CO_2$ molecules.

| $\sigma_C$ (nm) | $\sigma_O$ (nm) | $\epsilon_C$ (kJ/mol) | $\epsilon_O$ (kJ/mol) | $q_C$ (e) | $q_O$ (e) | $d_{CO}$ (nm) |
|---|---|---|---|---|---|---|
| 0.280 | 0.305 | 0.224 | 0.657 | 0.70 | -0.35 | 1.160 |

MD simulations with enhanced sampling are carried out using the PLUMED package (version 2.8.1) patched into the MD engine.[S7] The well-tempered metadynamics approach is used,[S8] where a bias potential of 10 kJ/mol was deposited every 250 fs with a width of $\frac{2}{256}$. The virtual temperature in metadynamics is set to 450 K, with a bias factor of 200. To prevent extreme deformation of the simulation box, additional restraints were introduced. Specifically, a penalty potential ($U_p$) was imposed whenever any of the box dimensions (X, Y, or Z) exceeded 5.0 nm or fell below 1.7 nm:

$$U_{p_l} = \begin{cases} 1500 \times (l - 1.7)^2, \text{ if l<1.7} \\ 1500 \times (l - 5.0)^2, \text{ if l>5.0} \\ 0, \text{ if 1.7<l<5.0} \end{cases} \tag{S1}$$

where $l$ represents the box length of the X, Y, or Z direction. An additional constraint on the total volume ($V$) was defined as

$$U_{p_V} = 1500 \times (V - 11.5)^2, \quad \text{if } V > 11.5\,\text{nm}^3. \tag{S2}$$

Intramolecular orientation was chosen as collective variables (CVs), which captures the relative alignment between a given molecule and its neighbors. The CV compares these orientations to predefined target values in order to identify. [S1, S9]

Two such CVs, $\lambda_1$ and $\lambda_3$, measure the average similarity of each $CO_2$ molecule to Phases I and III, respectively. The CV is defined as

$$\lambda = \sum_i^N \Gamma_i / N, \tag{S3}$$

where $N = 256$ and $\Gamma_i$ is the similarity of molecule $i$:

$$\Gamma_i = \frac{\rho_i}{n_i} \sum_j^N f_{ij} \Theta_{ij}, \tag{S4}$$

with $\rho_i$ and $n_i$ determined by coordination number:

$$\rho_i = 1/[1 + e^{-b(n_i - n_{cut})}], n_i = \sum_{j \neq i} f_{ij} \tag{S5}$$

The term $f_{ij}$ represent the continuous coordination weights,

$$f_{ij} = \frac{1}{1 + e^{a(r_{cut} - r_{ij})}}, \tag{S6}$$

where $r_{ij}$ is the distance between molecule $i$ and $j$, and $r_{cut} = 0.8$ nm. While $\Theta_{ij}$ quantifies how closely the relative orientation of neighboring molecules matches a reference phase:

$$\Theta_{ij} = \sum_{k}^{k_{max}} e^{-\frac{(\theta_{ij}-\theta_k)^2}{2\sigma_k^2}}, \tag{S7}$$

where $k_{max} = 2$ because multiple angles can describe the same phase. The parameter $\Gamma_i$ approaches 1 if a molecule $i$ perfectly aligns with a particular solid phase, while $\Gamma_i = 0$ indicates no alignment. The relevant reference angles of $\theta_k$ and $\sigma_k$ are listed in Table S2.

TABLE S2. Values of $\theta_k$ and $\sigma_k$ to calculate CVs $\lambda_1$ and $\lambda_3$.

| | $\theta_1$ (rad) | $\theta_2$ (rad) | $\sigma_1 = \sigma_2$ (rad) | $n_{cut}$ | $r_{cut}$ (nm) |
|---|---|---|---|---|---|
| $\lambda_1$ | 1.23 | 1.90 | 0.25 | 5 | 0.4 |
| $\lambda_3$ | 0.14 | 3.00 | 0.20 | 5 | 0.4 |

The free energy surface (FES), $F(\lambda_1, \lambda_3)$, was obtained using the PLUMED tool *sum_hills*. To determine the free energy difference from Phase I to Phase III ($\Delta G_{I\_III}$), we first defined the phase boundaries (Table I), as illustrated in the FES (Fig. S2). CV values $(\lambda_1, \lambda_3)$ outside the I/III regions were assigned to a liquid or amorphous phase. Finally, $\Delta G_{I\_III}$ was calculated using:

$$\Delta G_{I\_III} = -RT \ln \frac{P(III)}{P(I)} = -RT \ln \frac{\iint_{(\lambda_1,\lambda_3)\in III} d\lambda_1 d\lambda_3 e^{-\frac{F(\lambda_1,\lambda_3)}{RT}}}{\iint_{(\lambda_1,\lambda_3)\in I} d\lambda_1 d\lambda_3 e^{-\frac{F(\lambda_1,\lambda_3)}{RT}}} \tag{S8}$$

### B. Data preparation for the input of Gen-TM

While phase similarity scores $\lambda_1$ and $\lambda_3$ serve as global descriptors to distinguish $CO_2$ Phases I and III, capturing molecular-level structural details is essential for providing expTM with an Ising-model-like representation. To achieve this, we use the molecule-wise order parameter $\Gamma$ (Eq. S4). The input data for expTM are stored as NumPy arrays with shape $(n, 2, 16, 16)$, where $n$ represents the number of selected configurations, the second dimension (2) corresponds to the $\Gamma$ values for Phases I and III, and the $(16 \times 16)$ grid maps the 256 molecules in each configuration. For each pressure condition, we select $10^5$ distinct configurations, weighting their occurrences according to the probability

$$P(\lambda_1, \lambda_3) = e^{-\frac{F(\lambda_1,\lambda_3)}{RT}} \tag{S9}$$

as illustrated in Fig. S3.

### C. Backmapping

The current expTM model can only generate data in CV space. To map generated CVs $(\lambda_1, \lambda_3)$ back to actual atomic configurations, we use a nearest-neighbor approach: specifically, we run through all possible pairs between the MD-simulated data and the expTM-generated CVs to find the smallest norm difference (Fig. S4). From each reference pressure

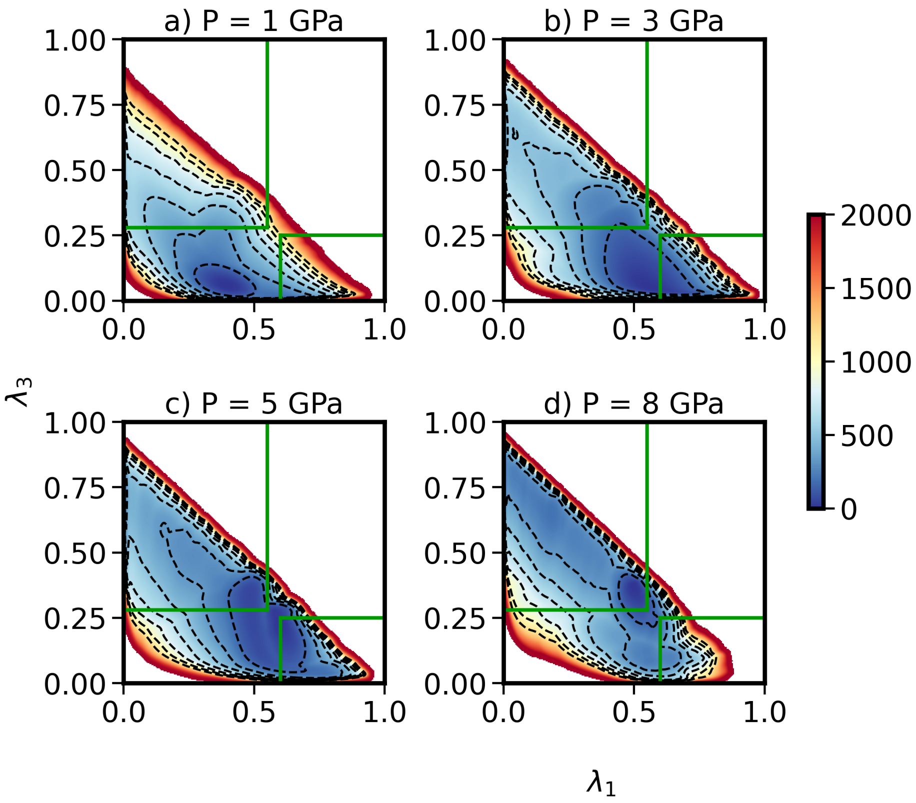


FIG. S2. Free energy surfaces (FES) calculated from MD simulations of $CO_2$ under different pressures. The minimum value of the free energy is set to 0. The unit for the color bar is kJ/mol. The CVs on the X and Y axes are $\lambda_1$ and $\lambda_3$, respectively. The color transitions to white where the free energy $F(\lambda_1, \lambda_3) > 2000$ kJ/mol. The green line indicates the regions corresponding to different phases, which remain consistent across simulations at all pressures, as described in the text. The top-left corner represents Phase III, while the bottom-right corner corresponds to Phase I.

$\left(P = 1\,\mathrm{GPa} \text{ and } P = 8\,\mathrm{GPa}\right)$, the generated points correctly match the characteristic structures observed in the real system (i.e., an alternating arrangement at low pressure and a linear arrangement at high pressure).

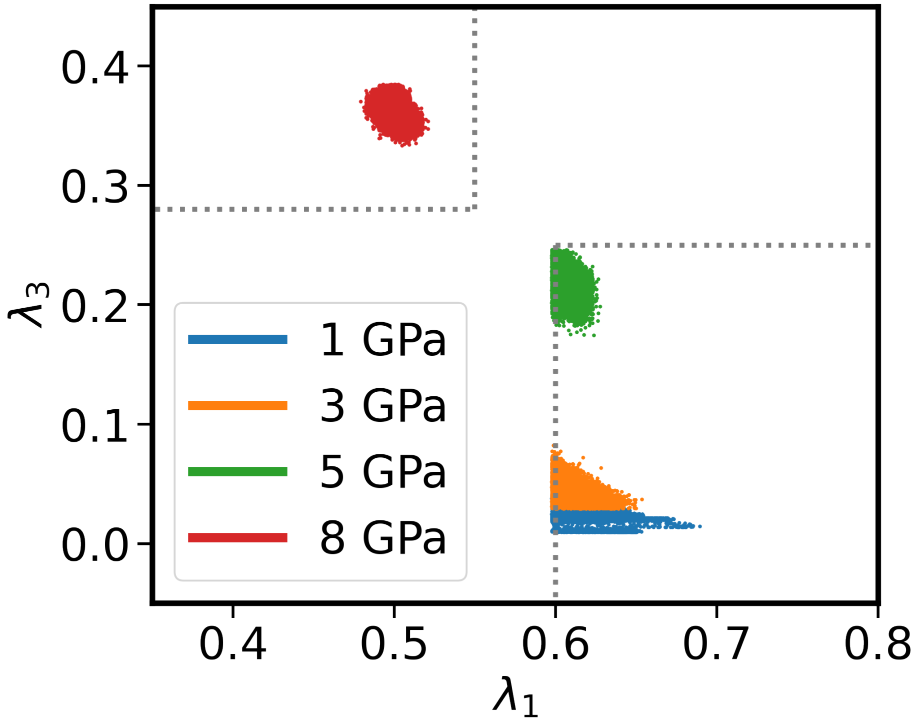


FIG. S3. Collective variable values ($\lambda_1$, $\lambda_3$) for the configurations used to train expTM. Each point represents the mean molecule-wise order parameters.

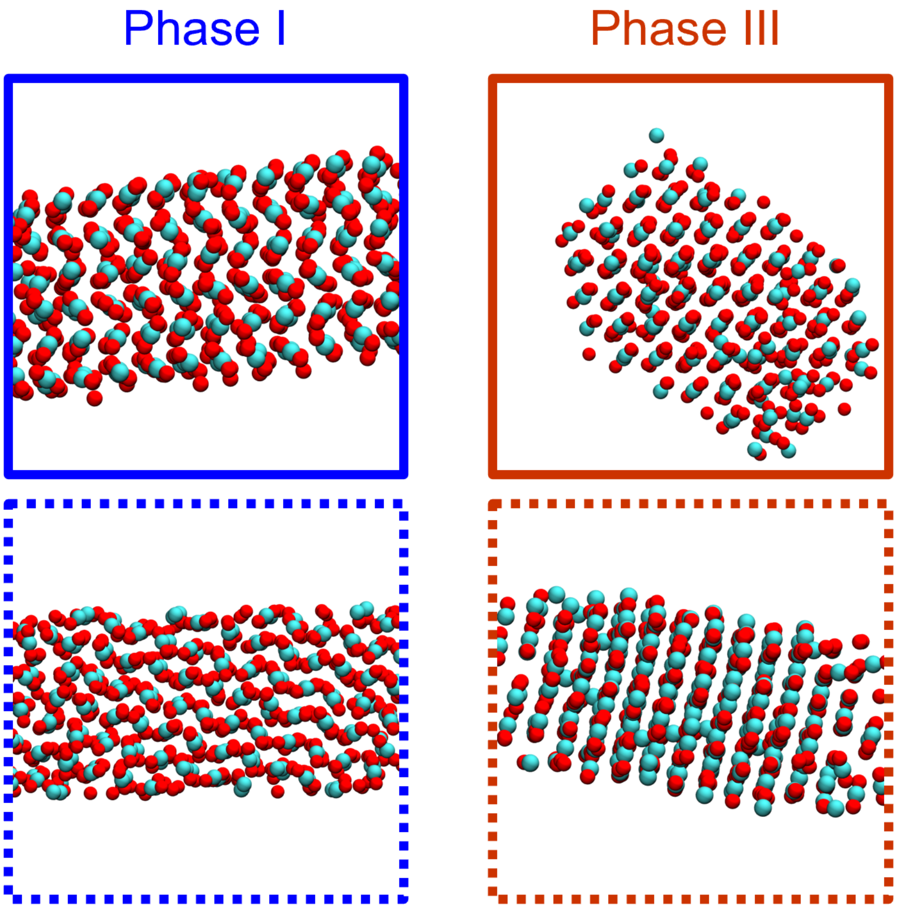


FIG. S4. Snapshots of $CO_2$ from MD simulations (top) and generated configurations via backmapping (bottom).

[S1] I. Gimondi and M. Salvalaglio, Co2 packing polymorphism under pressure: Mechanism and thermodynamics of the i-iii polymorphic transition, The Journal of chemical physics **147** (2017).

[S2] M. J. Abraham, T. Murtola, R. Schulz, S. Páll, J. C. Smith, B. Hess, and E. Lindahl, Gromacs: High performance molecular simulations through multi-level parallelism from laptops to supercomputers, SoftwareX **1**, 19 (2015).

[S3] S. Páll, M. J. Abraham, C. Kutzner, B. Hess, and E. Lindahl, Tackling exascale software challenges in molecular dynamics simulations with gromacs, in *Solving Software Challenges for Exascale: International Conference on Exascale Applications and Software, EASC 2014, Stockholm, Sweden, April 2-3, 2014, Revised Selected Papers 2* (Springer, 2015) pp. 3–27.

[S4] G. Bussi, D. Donadio, and M. Parrinello, Canonical sampling through velocity rescaling, The Journal of chemical physics **126** (2007).

[S5] H. J. Berendsen, J. v. Postma, W. F. Van Gunsteren, A. DiNola, and J. R. Haak, Molecular dynamics with coupling to an external bath, The Journal of chemical physics **81**, 3684 (1984).

[S6] B. Hess, P-lincs: A parallel linear constraint solver for molecular simulation, Journal of chemical theory and computation **4**, 116 (2008).

[S7] G. A. Tribello, M. Bonomi, D. Branduardi, C. Camilloni, and G. Bussi, Plumed 2: New feathers for an old bird, Computer physics communications **185**, 604 (2014).

[S8] A. Barducci, G. Bussi, and M. Parrinello, Well-tempered metadynamics: a smoothly converging and tunable free-energy method, Physical review letters **100**, 020603 (2008).

[S9] M. Salvalaglio, C. Perego, F. Giberti, M. Mazzotti, and M. Parrinello, Molecular-dynamics simulations of urea nucleation from aqueous solution, Proceedings of the National Academy of Sciences **112**, E6 (2015).
